# Supplementary material for: Regressing Transformers for Data-efficient Visual Place Recognition
Source: arXiv:2401.16304 source file (2024-01-29)
Supplement: Supplementary file 1 [file supp.tex]

\noindent\textbf{Descriptor distance function. }
The training scheme for VPR backbones that we propose can be generalized to learn a metric space for different distance metrics. 
In our experiments, we use the Euclidean distance, but also show the training of two transformer models using the Cosine distance as the metric function to compute descriptor distances in the latent space. We show the results that we obtained in Table~\ref{tab:metrics}, which indicate that Euclidean distance is a better choice than the Cosine distance for learning with both GCL and MSE functions for visual place recognition.

\begin{table}[!t]
\resizebox{\columnwidth}{!}{%
\begin{tabular}{@{}lllcccccc@{}}
\toprule
\multirow{2}{*}{\textbf{Encoder}} & \multirow{2}{*}{\textbf{Metric}} & \multirow{2}{*}{\textbf{Loss}} & \multicolumn{3}{c}{\textbf{MSLS-val}} & \multicolumn{3}{c}{\textbf{MSLS-test}} \\ \cmidrule(l){4-9} 
 &  &  & \textbf{R@1} & \textbf{R@5} & \textbf{R@10} & \textbf{R@1} & \textbf{R@5} & \textbf{R@10} \\ \midrule
ViT-R50 & Euclidean & GCL & 69.7 & 81.6 & 85.3 & 46.8 & 62.7 & 69.5 \\
ViT-R50 & Cosine & GCL & 64.9 & 80.5 & 84.5 & 43.9 & 59.0 & 65.5  \\
ViT-R50 & Euclidean & MSE & \textbf{82.6} & \textbf{91.1} & \textbf{93.6} & \textbf{61.8} & \textbf{77.2} & \textbf{80.7} \\
ViT-R50 & Cosine & MSE & 80.9 & 89.3 & 91.9 & 56.8 & 72.7 & 77.8 \\ \bottomrule
\end{tabular}%
}\caption{Comparison between equivalent models trained with a GCL~\cite{GCL} and an MSE (ours), using the Cosine and the Euclidean distance.}
\label{tab:metrics}
\end{table}
